# Supplementary material for: Complete Approximations of Incomplete Queries
Source: arXiv:2407.20932 source file (2024-07-30)
Supplement: Supplementary file 1 [file SuppMaterial-Sub28.tex]

%%%%%%%%%%%%%%%%%%%%%%% file typeinst.tex %%%%%%%%%%%%%%%%%%%%%%%%%
%
% This is the LaTeX source for the instructions to authors using
% the LaTeX document class 'llncs.cls' for contributions to
% the Lecture Notes in Computer Sciences series.
% http://www.springer.com/lncs       Springer Heidelberg 2006/05/04
%
% It may be used as a template for your own input - copy it
% to a new file with a new name and use it as the basis
% for your article.
%
% NB: the document class 'llncs' has its own and detailed documentation, see
% ftp://ftp.springer.de/data/pubftp/pub/tex/latex/llncs/latex2e/llncsdoc.pdf
%
%%%%%%%%%%%%%%%%%%%%%%%%%%%%%%%%%%%%%%%%%%%%%%%%%%%%%%%%%%%%%%%%%%%

\documentclass[runningheads,a4paper]{llncs}

%---------------------------------------------------------%
% PACKAGES %
%---------------------------------------------------------%
\input{../packages}

%% Footnotes-Listing %%

%----------------------------------------------%
% MARCOS
%----------------------------------------------%
\input{../macros/ogi-macros2.tex}        % stability
\input{../macros/ogi-magik-macros.tex}   % completeness
\input{../macros/ogi-macros-2017.tex}    % new macros for this paper
\input{../macros/julien-macros.tex}  % new macros for this paper
\input{../macros/ogi-new-macros.tex}  % new macros for this paper
\sloppy                 % fix overfull \hbox problems
%----------------------------------------------%

%---------------------------------------------------------%
% MACROS %
%---------------------------------------------------------%

%---------------------------------------------------------%

%---------------------------------------------------------%
% TITLE, AUTHORS, ETC %
%---------------------------------------------------------%
\title{Supplementary Material for the Paper:  
Complete Approximations of Incomplete Queries}
\titlerunning{Complete Approximations of Incomplete Queries}  
% abbreviated title (for running head)

% \newcommand{\authspace}{\hspace{1.5ex}}
\author{%
  % ~
Julien Corman \and 
Werner Nutt \and 
Ognjen Savkovi\'c 
% Ognjen Savkovi\'c$^{1}$\authspace%
% Evgeny Kharlamov$^{2}$\authspace%
% Werner Nutt$^{1}$\authspace%
% Pierre Senellart$^{3}$%
}       
\institute{
%1
    Free University of Bozen-Bolzano, Italy 
}

\begin{document}
\maketitle
\sloppy
\setcounter{tocdepth}{2}
\makeatletter
\renewcommand*\l@author[2]{}
\renewcommand*\l@title[2]{}
\makeatletter
\begingroup
\let\clearpage\relax
\tableofcontents
\endgroup
%---------------------------------------------------------%
% INPUTS
%---------------------------------------------------------%
%
% \newpage

\section{Overview}
This document contains the proofs omitted from the submitted version due to space limitations.
As in the paper, we assume that all queries are conjunctive queries.

% The proofs are grouped in sections based on the issue they are covering.

\input{SuppMaterial-Content}

\bibliographystyle{plain} % the recommended bibstyle
{\footnotesize
\bibliography{../bib/ognjen-bib,../bib/ognjen-new,../bib/os-bib,../bib/ref-stability}}

\end{document}
